# Supplementary material for: Iterative Depth-First Search for Fully Observable Non-Deterministic Planning
Source: arXiv:2204.04322 source file (2022-06-20)
Supplement: Supplementary file 1 [file supplementary_material.tex]

\section*{Supplementary Material}

We now formally present the theoretical proofs related to the \IDFS algorithm (not \IDFSSatisficing) presented in Algorithm~\ref{alg:IDFS}.
Here, we prove that \IDFS is \emph{sound} and \emph{complete} when the used heuristic function $h$ is \emph{admissible} and the evaluation function $\F$ is ``optimistic'' (i.e., $\F_{\min}$). A heuristic is admissible iff $h(s) \in \mathbb{Z}_{\geq 0} \cup \lbrace \infty \rbrace$ and $h(s)$ is a ``non-pessimistic'' estimation of the real minimum distance from a state $s$ to any goal state.

%------------------------------------------------------------------------

For proving \emph{soundness} and \emph{completeness} of our \IDFS algorithm, we formally prove that:
\begin{enumerate}
    \item \IDFSSearch \textbf{always terminates};
    \item \IDFSSearch \textbf{returns a solution} $\pi$ that is a strong cyclic solution for a \FOND planning task $\Pi$ with $\bound > \cv^*$, when a task $\Pi$ is \emph{solvable}; and
    \item \IDFSSearch \textbf{never returns a solution}, when a \FOND planning task $\Pi$ is \emph{unsolvable}.
\end{enumerate}

This supplementary material is structured as follows. We first prove that the \IDFS algorithm always terminates (Lemma~\ref{lem:increasing_bound}). Then, we prove that \IDFSSearchRec does not return false positives (Lemmas~\ref{lem:no_false_positives} and~2.1), i.e., it never returns a solution that is not a strong cyclic solution. Finally, we prove that, when it returns false negatives (\unsolved, but there is actually a solution), the new $bound$ is yet at most the \textit{minimal critical-value} $\cv^*$ (Lemmas~\ref{lem:no_false_negatives}, 3.1~and~3.1.1).

Our theoretical proofs are meant to be proved in a \emph{top-down} scheme. Claims~1 and~2 broadly introduce the conclusions and deductions that the Lemmas will lead to, before we formally prove them. 
We also provide some auxiliary Lemmas that are used in the proof of main Lemmas. The auxiliary Lemmas are placed after the Lemmas they are used on. Finally, we provide a Theorem that consolidates the theoretical proofs regarding the \emph{soundness} and \emph{completeness} of the \IDFS algorithm (Algorithm~\ref{alg:IDFS}).

\begin{claim}
Lemma~\ref{lem:increasing_bound} guarantees that \IDFS always terminates.
\end{claim}
\emph{Proof.} To prove that \IDFS always terminates, we need to prove that all loops of the algorithm have a finite number of iterations, and that all recursions of the algorithm have a finite depth. 
The while-loop continues only if the \emph{bound} is at most $|\S|$ (which is finite), thus, it has a finite number of iterations according to Lemma~\ref{lem:increasing_bound}. 
The repeat-loop has at most $|\succs(s,a)|+1$ iterations until reaching a fixed-point, because each iteration increases the size of $\solvedsuccessorsset$ to avoid reaching a fixed-point, and the size of $\solvedsuccessorsset$ is limited by $\succs(s,a)$ (which is finite). 
The for-loop iteration is limited by the size of $\succs(s,a)$ as well. Finally, the recursion depth is bounded by $|\S|+1$ because \IDFSSearchRec prevents state cycling.~$\hfill\blacksquare$

\begin{lemma} \label{lem:increasing_bound}
After a while-loop iteration, the value of the variable $\bound$ strictly increases by at least one.
\end{lemma}
\emph{Proof.} Before starting a while-loop iteration, the \emph{bound} is a finite integer number, because if it is $\infty$, there would be no iteration due to the while-loop termination condition, and because the first bound is in $\mathbb{Z} \cup \lbrace \infty \rbrace$ and the $\newbound$ variable is never set by $\IDFSSearchRec$ to a finite non-integer number. 
Therefore, any increase of $\bound$ would be of at least one. 
Moreover, since $\newbound$ is set as $\infty$ before starting a while-loop iteration, and it is never updated by $\IDFSSearchRec$ to a value that is not greater than the current bound (due to the if-statements conditions), then at the end of a while-loop iteration, it is always greater than $\bound$, increasing its value by at least one.~$\hfill\blacksquare$

\begin{claim}
Given that \IDFS always terminates, proving the following Lemmas~\ref{lem:no_false_positives} and~\ref{lem:no_false_negatives} is sufficient to guarantee the soundness and completeness of the algorithm. 
\end{claim}
\emph{Proof.} Lemma~\ref{lem:no_false_positives} guarantees that when the task is unsolvable, no solution will be ever returned.  Lemma~\ref{lem:no_false_negatives} guarantees that when the task is solvable, the flag $\solved$ is returned while $\bound \leq \cv^*$, which is before the while-loop termination condition is achieved, since $\cv^* \leq |\S|$, and the Lemma~\ref{lem:no_false_positives} also guarantees that, when that occurs, the returned policy is indeed a strong cyclic solution for a \FOND planning task $\Pi$.~$\hfill\blacksquare$

%------------------------------------------------------------------------

\newpage

%------------------------------------------------------------------------
\subsection*{No-false-positives' Realm}

In this section, we prove that \IDFSSearchRec does not return \textit{false positives} solutions, i.e., we formally prove (Lemmas~\ref{lem:no_false_positives} and~2.1) that \IDFSSearchRec never returns a solution that is not a strong cyclic solution for a \FOND planning task $\Pi$.

Before we proceed to formally define some key definitions and terminologies, we first introduce three useful notations:
\begin{itemize}
    \item $\S_*$ refers to the set of states $\lbrace s \mid s \models s_* \rbrace$;
    \item $S(\pi)$ refers to the states covered by a policy $\pi$; and
    \item $\pi+s:a$ refers to a policy $\pi$ extended with the mapping $\pi(s) = a$.
\end{itemize}

\begin{definition}
    A $\pi$-trajectory is a non-empty sequence of states $\langle s_1, s_2, \dots, s_k \rangle$ with $s_{i+1} \in \succs(s_i, \pi(s_i)), \forall i \in \lbrace 1, 2, \dots, k-1 \rbrace$. Its length is $k - 1$, and it is called empty iff its length is zero (i.e., iff its sequence of states contains a single state).
    
    The union of two $\pi$-trajectories $\omega_a = \langle s_{a1}, s_{a2}, \dots, s_{ax} \rangle$ and $\omega_b = \langle s_{b1}, s_{b2}, \dots, s_{by} \rangle$, is the $\pi$-trajectory $\omega_1^\frown\omega_2 = \langle s_{a1}, s_{a2}, \dots, s_{ax}, s_{b2}, \dots, s_{by} \rangle$. The union is not possible if $s_{ax} \neq s_{b1}$.
\end{definition}

\begin{definition}
A policy $\pi$ is \textbf{sinking} to a set of states $T$ iff any non-empty $\pi$-trajectory ends in a state $s'$ such that exists another (possibly empty) $\pi$-trajectory starting from $s'$ ending in a state of $T$.
\end{definition}

\begin{definition}
A set of states $T$ is \textbf{reachable} from a state $s$ in a policy $\pi$ iff there is a $\pi$-trajectory (possibly empty) starting from $s$ ending in a state of $T$.
\end{definition}

\begin{definition}\label{def:policy_stronger}
A policy $\pi$ is a \textbf{strong cyclic policy} if $\pi$ is \textbf{sinking} to $\S_*$ and $s_0$ is either a goal node or is defined in $\pi$.
\end{definition}

Definition~\ref{def:policy_stronger} is stronger than the definition of \textit{strong cyclic policies} presented in the \textbf{Background} section. It guarantees that there are no states in $\pi$ that fails to sink to the goal, but that are unreachable from $s_0$, which could exist using the definition presented in the \textbf{Background}.

\begin{definition}\label{def:partial_strong_cyclic_policy_SM}
A policy $\pi$ is a \textbf{partial strong cyclic policy} from $s$ for a set of primary target states $T$ and a set of secondary target states $T_W$, iff $T$ is \textbf{reachable} from $s$ in $\pi$ and $\pi$ is \textbf{sinking} to $T_W$.
    
    We say $\pi \models \langle s, T, T_W \rangle$ iff $\pi$ is a partial strong cyclic policy from $s$ for $T$ and $T_W$.
\end{definition}

Definition~\ref{def:partial_strong_cyclic_policy_SM} formally re-defines what we call as \textit{partial strong cyclic policies}. It is slightly different compared to the one we presented in Definition~\ref{def:partial_cyclic_policy}, in order to be suitable for theoretical proofs we present here.

\begin{definition}
A policy $\pi$ is a \textbf{potential-partial strong cyclic policy} from $s$ for a set of primary target states $T$ and a set of secondary target states $T_W$, disregarding a set of transitions $X$, iff $T$ would be \textbf{reachable} from $s$ in $\pi$ and $\pi$ would be \textbf{sinking} to $T_W$, if we do not take into account as a $\pi$-transition the $\pi$-transitions that contain a transition of $X$.
    
A \textbf{transition} is a pair state-state. A $\pi$-trajectory $\omega$ contains a transition $\langle s_1, s_2 \rangle$ iff $s_1$ appears exactly before $s_2$ in $\omega$. We call \textbf{$X$-free} a $\pi$-trajectory that does not contain transitions of $X$.
    
We say $\pi \models \langle s, T, T_W, X \rangle$ iff $\pi$ is a potential-partial strong cyclic policy from $s$ for $T$, $T_W$ and $X$.
\end{definition}

\newpage

\begin{lemma}\label{lem:no_false_positives}
Whenever in some while-loop iteration the flag returned by \IDFSSearchRec is $\solved$, the returned policy $\upi$ is a strong cyclic policy.
\end{lemma}
\emph{Proof.} We can apply Lemma~2.1 on the root call of \IDFSSearchRec made by \IDFSSearch, which is $\IDFSSearchRec(s_0, \emptyset, \emptyset, \emptypolicy)$, since $S(\emptypolicy) \cap \emptyset = \emptyset$ and an empty policy is \textbf{sinking} to any set of states. We then know that the \textit{returned policy} $\upi$ has the property $\upi \models \langle s_0, T, T_W \rangle$, where $T = \S_* \cup \emptyset$ and $T_W = \S_* \cup \emptyset$. Since $T_W$ is equal to the set of goal states of $\Pi$, then the returned policy $\upi$ is a strong cyclic policy for $\Pi$.~$\hfill\blacksquare$

\ramon[inline]{I still need to read carefully Lemma 3. It will be the last one, it is too dense.}
\begin{sublemma1}\label{lem:no_false_positives_with_assumptions}
    If $\IDFSSearchRec(s, \ancestorsset, \ancestorsset_*, \dpi)$ returns $\solved$, $S(\dpi) \cap \ancestorsset = \emptyset$ and $\dpi$ is sinking to $T = \S_* \cup \ancestorsset_*$, then the returned policy, which we call here $\upi$, has the property $\upi \models \langle s, T, T_W \rangle$, with $T_W = \S_* \cup \ancestorsset$ and $S(\upi) \cap \ancestorsset = \emptyset$.

\end{sublemma1}
    \emph{Proof.} For this proof, we will make a structural induction on which return-statements of the algorithm was the one that returned the $\solved$ flag. There are two return-statements that return $\solved$ flags, one (in Line~\ref{alg:IDFS:solved_1}) that is a base case, and another  (in Line~\ref{alg:IDFS:solved_2}) that is recursive and will be our induction step. The former occurs iff $s$ is a goal state or $s$ is contained (covered) in the received policy $\dpi$ or $s$ is in the received set $\ancestorsset_*$. The latter is recursive because it only can occur if all the recursive calls, made on all states $s'$ successor of $s$ from some applicable action, returned the $\solved$ flag as well (and because that set of successor states is never empty).
    
    In other words, if the algorithm returned the flag $\solved$, it may or may not have needed to make recursive calls before returning that flag, but if it needed, then all its recursive calls must also have returned the flag $\solved$. The same argument applies on the recursive calls made, and so on. That ends up making sort of a ``tree of calls'', with all the calls of the tree returning the flag $\solved$. The base case is the leaf nodes of that tree, which are the ones that returned $\solved$ using the first mentioned return-statement and did not make recursive calls. The non-leaf nodes, on the other hand, returned $\solved$ using the second mentioned return-statement (the recursive one). We start proving that the Lemma is valid for the leaf nodes, and then we inductively prove that the Lemma is also valid for any given layer of the tree, if it is valid for the layers below that one.
    
    \textbf{Base Case.} The returned policy $\upi$ is equal to the received policy $\dpi$, as it is not modified until the first return-statement, and the condition-to-occur of the first return-statement ensures that $s \in T$. Since $s \in T$, and the policy $\upi = \dpi$ is sinking to $T \subseteq T_W$, it is then direct that $\upi \models \langle s, T, T_W \rangle$ and that $S(\dpi) \cap \ancestorsset = \emptyset$ implies $S(\upi) \cap \ancestorsset = \emptyset$.~$\hfill\square$
    
    \textbf{Inductive Step.} Now, we want to prove that the policy $\upi$, if returned by the recursive return-statement, has as well the property $\upi \models \langle s, T, T_W \rangle$ and $S(\upi) \cap \ancestorsset = \emptyset$. For the recursive return-statement to occur, the set $\solvedsuccessorsset$  must have been filled with the successors of $s$ in some order -- namely the order: $s^1, s^2, \dots, s^k$ (without loss of generality) --  when we are analyzing an action $a$ applicable on $s$.
    
    By induction hypothesis, we know that the policy $\upi^i$, returned from the recursion call that solved $s^i$, has $S(\upi^i) \cap (\ancestorswiths) = \emptyset$ and the property $\upi^i \models \langle s^i, T^i, T_W^i \rangle$, with $T^i = \S_* \cup \ancestorsset_*'$ and $T_W^i = \S_* \cup (\ancestorswiths)$, if certain conditions are satisfied. The conditions are that $S(\pi') \cap (\ancestorswiths) = \emptyset$ and that $\pi'$ must be sinking to $T^i$. That is true because the recursive call that solved $s^i$ passed as third parameter the variable $\ancestorsset_*'$, and the variable $\pi'$ as the fourth, and the statement of this Lemma is valid by induction to the recursive calls. It is, however, inconvenient the fact that the values of the variables $\ancestorsset_*'$ and $\pi'$ vary over time, so we instead call $\ancestorsset_*^i$ and $\dpi^i$ the values of $\ancestorsset_*'$ and $\pi'$ at the moment when the recursion call that solved $s^i$ was made. This way, we specify better the composition of the sets~$T^i$ and~$T_W^i$.
    
    Now, to prove that $\upi \models \langle s, T, T_W \rangle$ and $\upi \cap \ancestorsset = \emptyset$ when $\dpi$ is sinking to $T$ and $\dpi \cap \ancestorsset = \emptyset$, we need to prove that $\upi^k+s:a \models \langle s, T, T_W \rangle$ and $\upi^k+s:a \cap \ancestorsset = \emptyset$ when $\dpi$ is sinking to $T$ and $\dpi \cap \ancestorsset = \emptyset$, because $\upi$ is precisely the policy $\upi^k+s:a$. We will do that by doing an induction proof on $i$, proving for each $i \in \lbrace 1, 2, \dots, k \rbrace$ that $S(\upi^i) \cup T \supseteq Y^i$, $S(\upi^i) \cap (\ancestorswiths) = \emptyset$ and $\upi^i+s:a \models \langle s, T, T_W, X^i \rangle$, with $Y^i = \lbrace s_1, s_2, \dots, s_i \rbrace$ and $X^i = \lbrace \langle s, s^{i+1} \rangle, \langle s, s^{i+2} \rangle, \dots, \langle s, s^{k} \rangle \rbrace$. Note the importance of the fact that when $i = k$ we have $X^i = \emptyset$ since this way we have an induction proof's corollary that is exactly what we wanted before: $S(\upi^k+s:a) \cap \ancestorsset = \emptyset$ and $\upi^k+s:a \models \langle s, T, T_W \rangle$. Therefore, proving this new induction will conclude the Lemma's proof.
    
    Since now we have nested inductions, we call this latter induction as the internal one, and the former as the external one. The external induction can be seen as a vertical induction on the search tree (bottom-up, with the ``bottom layer'' already proven by now), and the internal induction can be seen as a horizontal induction on a specific layer of the search tree (between sibling nodes). Note that we can use the assumptions of the Lemma (e.g. that $\dpi$ was sinking to $T$) and of the external induction to prove the internal induction.
    
    We start proving the \textit{internal base case}, which is when $i = 1$. As stated before, we know (by external induction hypothesis) that the policy $\upi^1$, returned from the recursion call that solved $s^1$, has $S(\upi^1) \cap (\ancestorswiths) = \emptyset$ and the property of $\upi^1 \models \langle s^1, T^1, T_W^1 \rangle$, with $T^1 = \S_* \cup \ancestorsset_*^1$ and $T_W^1 = \S_* \cup (\ancestorswiths)$, if $\dpi^1$ is sinking to $T^1$ and $S(\dpi^1) \cap (\ancestorswiths) = \emptyset$. It is true the conditions of $\dpi^1$ sinking to $T^1$ and $S(\dpi^1) \cap (\ancestorswiths) = \emptyset$ because $\dpi^1 = \dpi$ and $\ancestorsset_*^1 = \ancestorsset_*$, and we know that $\dpi$ is sinking to $\S_* \cup \ancestorsset_*$ and $\dpi \cap (\ancestorswiths) = \emptyset$. It is true that $\ancestorsset_*^1 = \ancestorsset_*$ and $\dpi^1 = \dpi$ because the algorithm initializes the variables $\ancestorsset_*'$ and $\pi'$ with these values, and their values are not updated until a solved successor of $s$ was found, which wasn't yet the case, as $s^1$ is the first solved successor. Since $\ancestorsset_*^1 = \ancestorsset_*$ and $\dpi^1 = \dpi$, we also know that the policy $\upi^1$ also has the property of $\upi^1 \models \langle s^1, T, T_W \cup \s \rangle$. Therefore, the policy $\upi^1+s:a$ would have the property $\upi^1+s:a \models \langle s, T, T_W, X^1 \rangle$, as $X^1$ disregards all successors of $s$ from $a$ except $s^1$. That was one of the things we needed to prove. Other is that $S(\upi^1) \cup T \supseteq Y^i = \lbrace s^i \rbrace$, and we get the fact of $s^1 \in S(\upi^1) \cup T$ because $T$ is reachable from $s^1$ in $\upi^1$, what wouldn't be possible if $s^1 \not\in S(\upi^1) \cup T$. Finally, we have that $\upi^1+s:a \cap \ancestorsset = \emptyset$ because $\ancestorsset$ does not contain $s$, and $S(\upi^1) \cap \ancestorsset = \emptyset$ since $S(\upi^1) \cap (\ancestorswiths) = \emptyset$, concluding the proof.~$\hfill\circ$
    
    Now we prove the \textit{internal induction step} ($i > 1$). As stated before, we know (by external induction hypothesis) that the policy $\upi^i$, returned from the recursion call that solved $s^i$, has $S(\upi^i) \cap (\ancestorswiths) = \emptyset$ and the property of $\upi^i \models \langle s^i, T^i, T_W^i \rangle$, with $T^i = \S_* \cup \ancestorsset_*^i$ and $T_W^i = \S_* \cup (\ancestorswiths)$, if $\dpi^i$ is sinking to $T^i$ and $S(\dpi^i) \cap (\ancestorswiths) = \emptyset$. So, before concluding anything from that, let's first check whether $\dpi^i$ is indeed sinking to $T^i$ and $S(\dpi^i) \cap (\ancestorswiths) = \emptyset$. This policy $\dpi^i$, which was given as argument to the recursive call that solved $s^i$, is equal to the policy $\upi^{i-1}$, returned from the recursion call that solved $s^{i - 1}$, because the algorithm always updates the value of variable $\pi'$ to the policy returned from a successful recursion call. Now, to check whether $\dpi^i = \upi^{i-1}$ is indeed sinking to $T^i$ and $S(\upi^{i-1}) \cap (\ancestorswiths) = \emptyset$, we look at the properties we know for $\upi^{i-1}$ by internal induction hypothesis.
    
    We know that, by internal induction hypothesis, first that $S(\upi^{i-1}) \cup T \subseteq Y^{i-1}$, second that $S(\upi^{i-1}) \cap (\ancestorswiths) = \emptyset$ and third that $\upi^{i-1}+s:a \models \langle s, T, T_W, X^{i-1} \rangle$. This second information is exactly the second thing we wanted to check about $\upi^{i-1}$, so remains for we check whether $\upi^{i-1}$ is indeed sinking to $T^i$. To do that, we look at the information that says that $\upi^{i-1}+s:a \models \langle s, T, T_W, X^{i-1} \rangle$. It turns out that it implies that $\upi^{i-1}$ is sinking to $T_W$, here's why: First, we know that $s$ is not part of $T_W = \S_* \cup \ancestorsset$, otherwise the execution of \IDFSSearchRec would have returned before the return-statement of the Line~\ref{alg:IDFS:solved_2}, what would violate the prime assumption of this external induction step. Second, we know that $s$ is not part of $\upi^{i-1}$ either, since $S(\upi^{i-1}) \cap (\ancestorswiths) = \emptyset$, as stated in the beginning of this paragraph. Therefore, all $\upi^{i-1}$-trajectories are also $\upi^{i-1}+s:a$-trajectories. Thus, the fact that $\upi^{i-1}+s:a$ is sinking to $T_W$ under some disregardances about transitions outgoing $s$ implies that $\upi^{i-1}$ is also sinking to $T_W$ independently of such disregardances, since $s \not\in S(\upi^{i-1}) \cup T_W$, and thus the transitions outgoing $s$ are completely irrelevant for this analysis. Now, since $T^i = \S_* \cup \ancestorsset_*^i \supseteq \S_* \cup \ancestorsset = T_W$ -- because $\ancestorsset_*^i = \ancestorswiths$ for all $i > 1$, as the algorithm always updates the value of variable $\ancestorsset_*'$ to $\ancestorswiths$ when a recursion call returns successfully --, we know that $\upi^{i-1}$ is as well sinking to $T^i$, which is exactly the condition that remained to us to check. Since now we confirmed that $\dpi^i = \upi^{i-1}$ is indeed sinking to $T^i$ and $S(\dpi^i) \cap (\ancestorswiths) = \emptyset$, we really know now that the policy $\upi^i$, returned from the recursion call that solved $s^i$, has $S(\upi^i) \cap (\ancestorswiths) = \emptyset$ and the property of $\upi^i \models \langle s^i, T^i, T_W^i \rangle$, and we will use this knowledge to prove what we needed from the beginning: first that $S(\upi^i) \subseteq Y^i$, second that $S(\upi^i) \cap (\ancestorswiths) = \emptyset$ and third that $\upi^i+s:a \models \langle s, T, T_W, X^i \rangle$. Note, however, that the second is already done, so it only remains for we prove that $S(\upi^i) \cup T \subseteq Y^i$ and $\upi^i+s:a \models \langle s, T, T_W, X^i \rangle$.
    
    It is almost direct that $S(\upi^i) \cup T \subseteq Y^i$, since $\upi^i$ was built upon $\upi^{i-1}$ (thus $S(\upi^i) \subseteq S(\upi^{i-1})$) and since $S(\upi^{i-1}) \cup T \subseteq Y^{i-1}$. With just this information, we know that $S(\upi^i) \cup T \subseteq S(\upi^{i-1}) \cup T \subseteq Y^{i-1} = Y^i \setminus \lbrace s^i \rbrace$. It only remains to prove that $s^i \in S(\upi^i) \cup T$. We know that $\upi^i \models \langle s^i, T^i, T_W^i \rangle$, with $T^i = \S_* \cup \ancestorsset_*^i$. Now, since $T^i$ is reachable from $s^i$ in $\upi^i$ and $T^i \subseteq T$, it must be true that $s^i \in S(\upi^i) \cup T^i$ and thus that $s^i \in S(\upi^i) \cup T$, concluding the proof that $S(\upi^i) \cup T \subseteq Y^i$ so it only remains for we prove that $\upi^i+s:a \models \langle s, T, T_W, X^i \rangle$.

    To prove that $\upi^i+s:a \models \langle s, T, T_W, X^i \rangle$, we need to prove that $T$ is reachable from $s$ in $\upi^i+s:a$ disregarding $X^i$ and that $\upi^i+s:a$ is sinking to $T_W$ disregarding $X^i$. Since we know that $T^i$ is reachable from $s^i$ in $\upi^i$ (because $\upi^i \models \langle s^i, T^i, T_W^i \rangle$), and since $T^i = \S_* \cup \ancestorsset_*^i = \S_* \cup (\ancestorswiths) \supseteq \S_* \cup \ancestorsset \supseteq \S_* \cup \ancestorsset_* = T$, we then know that $T$ is reachable from $s^i$ in $\upi^i$, and thus $T$ is also reachable from $s$ in $\upi^i+s:a$, even without disregarding anything, which is stronger. Thus, only remains for we to prove that $\upi^i+s:a$ is sinking to $T_W$ disregarding $X^i$.
    
    We will make this final proof by contradiction, i.e., assuming that $\upi^i+s:a$ is \emph{not} sinking to $T_W$ even disregarding $X^i$. Meaning that there must be at least one non-empty $\upi^i+s:a$-trajectory ending in a state $s'$, such that there is no $\upi^i+s:a$-trajectory (even empty) starting from $s'$ ending in a state of $T_W$. We call the $\upi^i+s:a$-trajectories with this property as $T_W$-leavers. We select one such $T_W$-leaver $\upi^i+s:a$-trajectory and call it $\omega$. If $\omega$ is not $X^i$-free, we select another $T_W$-leaver $\upi^i+s:a$-trajectory. There must be one that is $X^i$-free, otherwise $\upi^i+s:a$ would be sinking to $T_W$ disregarding $X^i$. If $\omega$ ends in $s$, $\omega^\frown \langle s, s^i \rangle$ is also a $T_W$-leaver $\upi^i+s:a$-trajectory. Suppose otherwise, then there is a $\upi^i+s:a$-trajectory $\omega'$ (possibly empty) starting from $s^i$ ending in a state of $T_W$. Note then, that $\langle s, s^i \rangle^\frown\omega'$ would be a $\upi^i+s:a$-trajectory starting from the end state of $\omega$ ending in a state of $T_W$, contradicting the fact that $\omega$ is $T_W$-leaver. Now, if the selected $\omega$ ends in $s$, we replace it by $\omega^\frown \langle s, s^i \rangle$. Now, $\omega$ is guaranteed to not end in $s$ and is still $X^i$-free. Note that since $\omega$ is non-empty, we can obtain a $\upi^i+s:a$-trajectory $\omega_{\text{tail}}$ by removing all but the last two states of $\omega$. The resulting trajectory is also $T_W$-leaver, by the definition of being $T_W$-leaver, since they both have the same end state. Thus, if our selection gave us a $X^i$-free $T_W$-leaver $\upi^i+s:a$-trajectory $\omega$ with length greater than $1$, we can replace it by $\omega_{\text{tail}}$. Now $\omega$ is guaranteed to not end in $s$ and have size one. Thus $\omega$ is of the form of $\langle s_x, s_y \rangle$, with $a' = (\upi^i+s:a)(s_x)$, $s_y \in \succs(s_x, a')$ and $s_y \not\in (T_W \cup \s)$.
    
    If $s_x$ is not $s$, $\omega$ is a $\upi^i$-trajectory, because it is a $\upi^i+s:a$-trajectory. But if $\omega$ is a $\upi^i$-trajectory, $\omega$ is not $T_W^i$-leaver, because $\upi^i$ is sinking to $T_W^i$. Now, since $T_W^i = \S_* \cup (\ancestorswiths)$ and $T_W = \S_* \cup \ancestorsset$, $\omega$ being $T_W$-leaver but not $T_W^i$-leaver, implies that there is a $\upi^i$-trajectory $\omega'$ starting from $s_y$ ending in a state of $T_W^i \setminus T_W = \s$, which must be $s$. Since $S(\upi^i) \cap (\ancestorswiths) = \emptyset$, we know that $\upi^i(s) = \bot$ and thus, $\omega'$ is $X^i$-free. Since all $\upi^i$-trajectories are $\upi^i+s:a$-trajectories, $\omega'$ is $\upi^i+s:a$-trajectory. By the same arguments as used before, $\omega'$ must be $T_W$-leaver, otherwise $\omega$ would not be $T_W$-leaver. And also by the same arguments as before, we can replace $\omega$ by $\omega'$, then $\omega'$ by $\omega'^\frown \langle s, s^i \rangle$, and finally $\omega'^\frown \langle s, s^i \rangle$ by $(\omega'^\frown \langle s, s^i \rangle)_{\text{tail}}$. By doing all this procedure, we start from $\omega$ not starting from $s$, and replace it by another $X^i$-free $T_W$-leaver $\upi^i+s:a$-trajectory $\omega$ not ending in $s$, with length $1$, but now \emph{guaranteed to start from $s$}. Thus $\omega$ is now of the form of $\langle s, s_y \rangle$, with $s_y \in \succs(s, a)$ and $s_y \not\in (T_W \cup \s)$. Since $\omega$ is $X^i$-free, $s_y \in \lbrace s^1, s^2, \dots, s^i \rbrace$.
    
    Let's consider that $s_y \neq s^i$. Then, $\omega$ is $X^{i-1}$-free and $s_y \in Y^{i-1} = \lbrace s^1, s^2, \dots, s^{i-1} \rbrace$. We know that, by internal induction hypothesis, $\upi^{i-1}+s:a \models \langle s, T, T_W, X^{i-1} \rangle$ and that $S(\upi^{i-1}) \cup T \subseteq Y^{i-1}$. Since $\upi^{i-1}+s:a$ is sinking to $T_W$ disregarding $X^{i-1}$, we know that all $X^{i-1}$-free $\upi^{i-1}+s:a$-trajectories are not $T_W$-leavers. If $s_y \in S(\upi^{i-1})$, $\omega$ would not be $T_W$-leaver as well, because there is at least one $X^{i-1}$-free $\upi^{i-1}+s:a$-trajectories $\langle s_y, s' \rangle$ with $s' \in \succs(s_y, (\upi^{i-1}+s:a)(s_y))$ that is not $T_W$-leaver, and because all $\upi^{i-1}+s:a$-trajectories are $\upi^i+s:a$-trajectories, since $\upi^i$ was built upon $\upi^{i-1}$. If $\omega$ is not $T_W$-leaver, there is a contradiction. Thus, we know that $s_y \not\in S(\upi^{i-1})$. But we also know that $S(\upi^{i-1}) \cup T \subseteq Y^{i-1}$ and $s_y \in Y^{i-1}$. Therefore $s_y \in T$. Since $T = \S_* \cup \ancestorsset_* \subseteq \S_* \cup \ancestorsset = T_W$, then $s_y \in T_W$, but that is a contradiction with $\omega$ being $T_W$-leaver. Therefore, since assuming $s_y \neq s^i$ led us to contradictions, we know that $s_y$ must be $s^i$. Thus, $\omega$ is $\langle s, s^i \rangle$ while $T_W$-leaver.
    
    Since we know that $T^i$ is reachable from $s^i$ in $\upi^i$, because $\upi^i \models \langle s^i, T^i, T_W^i \rangle$, we then know there is a $\upi^i$-trajectory $\omega'$ starting from $s^i$ ending in a state of $T^i$. Since all $\upi^i$-trajectories are $\upi^i+s:a$-trajectories, $\omega'$ is $\upi^i+s:a$-trajectory. By the same arguments as used before, $\omega'$ must be $T_W$-leaver, otherwise $\omega$ would not be $T_W$-leaver. Since $T^i = \S_* \cup \ancestorsset_*^i = \S_* \cup (\ancestorswiths)$ and $T_W = \S_* \cup \ancestorsset$, we then know that $\upi^i$-trajectory $\omega'$ starting from $s^i$ ending in a state of $T_W^i \setminus T_W = \s$, which must be $s$. Thus $\omega^\frown\omega'$ is $T_W$-leaver and ends in $\s$. Before we continue, take a special note that this $T_W$-leaver $\upi^i+s:a$-trajectory $\omega^\frown\omega'$ must exist, because if it not exist, we would have a contradiction to our assumption that $\upi^i+s:a$ is \emph{not} sinking to $T_W$ even disregarding $X^i$, since we considered all the possibilities of $\omega$, and they all either lead us to here or to a contradiction.
    
    Since $\upi^{i-1}+s:a \models \langle s, T, T_W, X^{i-1} \rangle$, we know that there is a $\upi^{i-1}+s:a$-trajectory $\omega''$ starting from $s$ ending in $T$. Since all $\upi^{i-1}+s:a$-trajectories are $\upi^i+s:a$-trajectories, since $\upi^i$ was built upon $\upi^{i-1}$, we have that $\omega''$ is also a $\upi^i+s:a$-trajectory. Since $T = \S_* \cup \ancestorsset_* \subseteq \S_* \cup \ancestorsset = T_W$, $\omega''$ is starting from $s$ ending in $T_W$. Thus $\omega^\frown\omega'^\frown\omega''$ is ending in $T_W$, contradicting with the fact that $\omega^\frown\omega'$ was $T_W$-leaver. Therefore $\upi^i+s:a$ must, by contradiction, be sinking to $T_W$ disregarding $X^i$, concluding our proof.~$\hfill\circ$
    
    $\hfill\square$
    
    $\hfill\blacksquare$
    
\newpage

%------------------------------------------------------------------------
\subsection*{No-false-negatives' Realm}

In this section, we formally prove that, when \IDFSSearchRec returns \textit{false negatives} (\unsolved, but there is actually a solution), the new $bound$ is yet at most the \textit{minimal critical-value} $\cv^*$ (Lemmas~\ref{lem:no_false_negatives}, 3.1~and~3.1.1).

In the \textbf{Minimal Critical-Value in \FOND Planning} section, we define that, if \IDFS uses $\minF$ and an admissible heuristic function for the deterministic version of the task~$\Pi$, \IDFS will search to a depth of at most the \emph{minimal critical-value} $\cv^*$. As we formally defined in Definitions~\ref{def:st} and \ref{def:cv*}, recall that the \textbf{critical-value} $\cv(\pi)$ of a policy $\pi$ is the value of the length of the longest $\pi$-trajectory $\langle s^1, s^2, \dots, s^k \rangle$ with $s^1 = s_0$ and no $i < j \leq k - 1$ with $s^i = s^j$, whereas 
the \textbf{minimal critical-value} $\cv^*$ of a \FOND planning task $\Pi$ is equal to $\min_{\pi \in \P(\Pi)} \cv(\pi)$. 
We define $\pi_*$ as a solution policy for a \FOND planning task $\Pi$ that has a minimal critical-value $\cv^*$, namely, $\cv(\pi_*) \in \min_{\pi \in \P(\Pi)} \cv(\pi)$, i.e., $\cv(\pi_*) = \cv^*$.
We denote the \textit{maximal} (\emph{longest}) $\pi_*$-trajectories outgoing from $s_0$ in the graph\footnote{Solution policies can be represented as standard directed graphs, as we illustrate in
Figures~\ref{fig:critical_value_policy}c and~\ref{fig:critical_value_policy}b, the graphs for the policies $\pi_0$ and $\pi_1$, respectively.} of $\pi_*$ as ``\textit{trails}'' henceforth.

These characterizations are useful for the the Lemmas~\ref{lem:no_false_negatives}, 3.1, and~3.1.1.    
We know from the definition of $\cv$s that all trails of a policy $\pi$ have size at most $\cv(\pi)$. 
We also know that some of the trails end up in a goal state, which we call as ``trails of \textit{Kind} $1$'', and that there may exist other trails that do not end up in a goal state, but loops (by means of cycles) in a state of itself. 
We call a trail to be of \textit{Kind} $k$ (for $k > 1$) if it ends up in a state $s$ of itself, such that $s$ is also part of another trail whose \textit{Kind} $k' = k-1$ but is not part of a trail of \textit{Kind} $k'' \leq k-2$. All trails of a strong cyclic solution $\pi$ have some \textit{Kind} $k$ associated to it, because no trail is a dead-end trail and all of them indeed end up in a goal state or loops in itself (thus no sort of trail is missed).
    
As we mentioned before, a state $s$ can be part of multiple trails, so we define its \textit{Kind} to be the \textbf{minimum} \textit{Kind} among the \textit{Kind}s of the multiple trails it belongs to, with one exception: we call the goal states to be of \textit{Kind} $0$. It conveniently guarantees that a trail of \textit{Kind} $k$ ends up in a state of \textit{Kind} $k-1$. As a matter of notation, we use $K(s)$ and $K(t)$ to specify the \textit{Kind} of a state and a trail, respectively. Figure~\ref{fig:Kind} exemplifies the notion of our \emph{Kind}s for the trails in a strong cyclic solution.

\begin{figure}[!ht]
	\centering
	\begin{tikzpicture}[
        node distance=10mm and 10mm, on grid, auto, label distance=-0.5mm,
        black_node/.style={draw=black, fill=white, very thick, circle}
        ]

        \node[accepting, black_node] (*) {\small$s_{\Omega}$} ;
        
        \node[initial above, initial text=, black_node] (A_0) [right = of *] {\small$s_{A0}$} ;
        \node[black_node] (A_1) [below = of A_0] {\small$s_{A1}$} ;
        \node[black_node] (A_2) [below = of A_1] {\small$s_{A2}$} ;
        \node[black_node] (A_3) [below = of A_2] {\small$s_{A3}$} ;
        \node[black_node] (A_4) [below = of A_3] {\small$s_{A4}$} ;
        \node[black_node] (A_5) [below = of A_4] {\small$s_{A5}$} ;
        
        \node[black_node] (B_1) [right = of A_1] {\small$s_{B1}$} ;
        \node[black_node] (B_2) [below = of B_1] {\small$s_{B2}$} ;
        \node[black_node] (B_3) [below = of B_2] {\small$s_{B3}$} ;
        \node[black_node] (B_4) [below = of B_3] {\small$s_{B4}$} ;
        \node[black_node] (B_5) [below = of B_4] {\small$s_{B5}$} ;
        
        \node[black_node] (C_2) [right = of B_2] {\small$s_{C2}$} ;
        \node[black_node] (C_3) [below = of C_2] {\small$s_{C3}$} ;
        \node[black_node] (C_4) [below = of C_3] {\small$s_{C4}$} ;
        \node[black_node] (C_5) [below = of C_4] {\small$s_{C5}$} ;
        
        \node[black_node] (D_3) [right = of C_3] {\small$s_{D3}$} ;
        \node[black_node] (D_4) [below = of D_3] {\small$s_{D4}$} ;
        \node[black_node] (D_5) [below = of D_4] {\small$s_{D5}$} ;
        
        \node[black_node] (E_4) [right = of D_4] {\small$s_{E4}$} ;
        \node[black_node] (E_5) [below = of E_4] {\small$s_{E5}$} ;
        
        \node[black_node] (F_5) [right = of E_5] {\small$s_{F5}$} ;
        
        \draw[-Stealth] (A_0.south)      -- (A_1.north)      ;
        \draw[-Stealth] (A_1.south)      -- (A_2.north)      ;
        \draw[-Stealth] (A_2.south)      -- (A_3.north)      ;
        \draw[-Stealth] (A_3.south)      -- (A_4.north)      ;
        \draw[-Stealth] (A_4.south)      -- (A_5.north)      ;
        \draw[-Stealth] (A_5.west)       -- (*.south east)   ;
        
        \draw[-Stealth, draw=red] (A_0.east)       -- (B_1.north)      ;
        \draw[-Stealth, draw=red] (B_1.south)      -- (B_2.north)      ;
        \draw[-Stealth, draw=red] (B_2.south)      -- (B_3.north)      ;
        \draw[-Stealth, draw=red] (B_3.south)      -- (B_4.north)      ;
        \draw[-Stealth, draw=red] (B_4.south)      -- (B_5.north)      ;
        \draw[-Stealth, draw=red] (B_5.west)       -- (A_0.south east) ;
        
        \draw[-Stealth] (B_1.east)       -- (C_2.north)      ;
        \draw[-Stealth] (C_2.south)      -- (C_3.north)      ;
        \draw[-Stealth] (C_3.south)      -- (C_4.north)      ;
        \draw[-Stealth] (C_4.south)      -- (C_5.north)      ;
        \draw[-Stealth] (C_5.west)       -- (B_1.south east) ;
        
        \draw[-Stealth, draw=blue] (C_2.east)       -- (D_3.north)      ;
        \draw[-Stealth, draw=blue] (D_3.south)      -- (D_4.north)      ;
        \draw[-Stealth, draw=blue] (D_4.south)      -- (D_5.north)      ;
        \draw[-Stealth, draw=blue] (D_5.west)       -- (C_2.south east) ;
        
        \draw[-Stealth] (D_3.east)       -- (E_4.north)      ;
        \draw[-Stealth] (E_4.south)      -- (E_5.north)      ;
        \draw[-Stealth] (E_5.west)       -- (D_3.south east) ;
        
        \draw[-Stealth, draw=red] (E_4.east)       -- (F_5.north)      ;
        \draw[-Stealth, draw=red] (F_5.west)       -- (E_4.south east) ;
        
        \draw[-Stealth] (F_5.east) to [out=0, in=315, looseness=10] (F_5.south east) ;
        
    \end{tikzpicture}
	\caption{Graph example of strong cyclic solution with $\cv = 6$. The trail in blue has \textit{Kind} $4$.}
	\label{fig:Kind}
\end{figure}

\begin{lemma} \label{lem:no_false_negatives}
    If in some while-loop iteration \IDFSSearchRec returns $\unsolved$ and the next bound is greater than $\cv^*$, then the task is unsolvable.
\end{lemma}
\emph{Proof.} We prove the statement above by contradiction, assuming that the \FOND planning task $\Pi$ is actually solvable. 
If $\Pi$ is solvable, it has a strong cyclic policy $\pi_*$ with $\cv(\pi_*) = \cv^*$, and thus we can applying the following Lemma~3.1 on $s_0$ unless $s_0$ is a goal state. Since $K(s_0)$ is always equal to one when $s_0$ is not goal but the task is solvable. Note that if $s_0$ is a goal state, \IDFSSearchRec immediately returns the flag $\solved$, a direct contradiction.

By applying Lemma~3.1 on $s_0$, we know that $\IDFSSearchRec(s_0, \emptyset, \emptyset, \emptypolicy)$ either returns $\solved$ or decreases the $\newbound$ to a value not greater than $\cv^*$, but that is a contradiction with our initial hypothesis that it returned $\unsolved$ and the next bound is greater than $\cv^*$, implying that our assumption that the task was solvable was incorrect, so we conclude our proof by contradiction.~$\hfill\blacksquare$ 

\begin{sublemma2}\label{lem:k=1}
    $\IDFSSearchRec(s, \ancestorsset, \ancestorsset_*, \pi)$ either returns $\solved$ or decreases the $\newbound$ to a value not greater than $\cv^*$, given that:
    \begin{itemize}
        \item $K(s) = 1$; and
        \item $\ancestorsset$ contains the states in the directed simple $\pi_*$-trajectory from $s_0$ to $s$ in the graph (including $s_0$, but excluding $s$).
    \end{itemize} Considering the graph of a solution $\pi_*$ with $\cv(\pi_*) = \cv^*$.
\end{sublemma2}
\emph{Proof.} For this proof, we make an induction on $H(s)$, being $H(s)$ the size of the longest directed simple $\pi_*$-trajectory in the graph of $\pi^*$ from $s$ to a goal state. Note that $g(s) + H(s) \leq \cv(\pi_*) = \cv^*$, by definition of $\cv$s.

\paragraph{Base Case.} We start analyzing when $H(s) = 1$ (the minimal $H(s)$ possible since $s$ is not a goal state, as its \textit{Kind} is not zero).

We prove the base case by contradiction, assuming that $\IDFSSearchRec(s, \ancestorsset, \ancestorsset_*, \pi)$ does not return $\unsolved$ and does not decrease the $\newbound$ to a value not greater than $\cv^*$. Since $s$ is not in $(\ancestorsset \setminus \ancestorsset_*)$, the $\unsolved$ flag must have been returned in the last line of \IDFSSearchRec, meaning that it analyzed all actions applicable in $s$, and failed to find one that solves $s$, including the action $\pi_*(s)$. Let's see what happens when the for-loop analyzed the action $\pi_*(s)$.

We know that $g(s) \leq \cv^* - H(s) = \cv^* - 1$, thus $g(s) + 1 \leq \cv^*$, meaning that the second if-continue statement will not be triggered, otherwise the $\newbound$ variable (which is never increased by \IDFSSearchRec) would be reduced to a value not greater than $\cv^*$, contradicting our initial hypothesis. 

We also know that $\F(\succs(s, \pi_*(s)))$ is at most $\cv^*$, due to the fact that we are using the $\minF$ heuristic estimation, and thus $\F(\succs(s, \pi_*(s))) = g(s) + 1 + \min_{s' \in \succs(s, \pi_*(s))}\lbrace h(s') \rbrace$, and also know that, since there is a goal state $s'$ successor of $s$ (with $h(s') = 0$ since we are using an admissible heuristic $h$), we know that $\F(\succs(s, \pi_*(s))) = g(s) + 1$, what is at most $\cv^*$ as just as stated above. Therefore, the first if-continue statement will not be triggered as well, and thus we know that the repeat-loop was reached.

Since the flag $\solved$ was not returned, we know that the recursive call on at least one successor state $s'$ of $s$ returned $\unsolved$. First, we know that $K(s')$ cannot be zero, due to the fact that if $s'$ is a goal state, the recursive call would return $\solved$ immediately, what would be therefore a contradiction. Furthermore, since $H(s) = 1$, we know that $K(s')$ cannot be equal to $K(s)$, otherwise $H(s) \geq H(s') + 1 \geq 1 + 1$ (contradicting $H(s) = 1$). Then, we conclude that $K(s')$ must be greater than $K(s) = 1$.

We know that $s$ has at least one successor $s''$ that is a goal state, and we already know that the recursive call on $s''$ returns the $\solved$ flag. Therefore, we know that at some point in the repeat-loop, the recursive call on $s'$ had $\ancestorsset_*' = \ancestorswiths$. Now, if we apply the following Lemma~2.1 on $s'$, we know that $\IDFSSearchRec(s', \ancestorswiths, \ancestorsset_*' = \ancestorswiths, \pi' \supseteq \pi)$ either returns $\solved$ or decreases the $\newbound$ to a value not greater than $\cv^*$. The first option is false because it would cause a direct contradiction. The second one is also false because the $\newbound$ variable has its value never increased by \IDFSSearchRec, and our initial hypothesis was that $\IDFSSearchRec(s, \ancestorsset, \ancestorsset_*, \pi)$ does not decrease the $\newbound$ to a value not greater than $\cv^*$. Thus, we conclude our proof by contradiction.~$\hfill\square$

\ramon{Frederico, please, double check this part.}
\paragraph{Induction Step.} We now analyze the induction step, which is the case when $H(s) > 1$. We also prove the induction step by contradiction, and, based on the same arguments we used for the base case, we find that the repeat-loop was reached for the action $\pi_*(s)$, and also that the recursive call on at least one successor state $s'$ of $s$ returned $\unsolved$. However, there is one difference here, spite of our argument, we know that $\F(\succs(s, \pi_*(s)))$ is at most equal to $\cv^*$. Now $s$ does not necessarily have a successor state $s'$ with $h(s') = 0$, but we know that if $s$ does not have one, it does not have goal successor states, and then it must have a successor state $s'$ of \textit{Kind} $1$, where such successor state $s'$ must have $h(s') \leq H(s') \leq \cv^* - g(s') =  \cv^* - (g(s) + 1)$, following to the same results that $\F(\succs(s, \pi_*(s))) \leq \cv^*$. Therefore, we can safely proceed with our analysis of the (non-necessarily unique) successor state $s'$ of $s$ whose recursive call returned $\unsolved$.

We already know that $s'$ cannot have $K(s') = 0$, otherwise, it would be a goal state and its recursive call would immediately return $\solved$. We also know, by the arguments of the base case, that $K(s')$ cannot be greater than $1$ as well. Thus our remaining case is to analyze what happens when $K(s') = 1$.

By induction step, we know that the recursive call on $s'$ either returns $\solved$ or decreases the $\newbound$ to a value not greater than $\cv^*$, since $H(s')$ must be lower to $H(s)$. And by the same arguments of the base case, that allow us to conclude our proof by contradiction.~$\hfill\square$

$\hfill\blacksquare$

\begin{sublemma3}\label{lem:k>1}
    $\IDFSSearchRec(s, \ancestorsset, \ancestorsset_*, \pi)$ either returns $\solved$ or decreases the $\newbound$ to a value not greater than $\cv^*$, given that:
    \begin{itemize}
        \item $K(s) \geq 2$;
        \item $\ancestorsset$ contains the states in the directed simple $\pi$-trajectory from $s_0$ to $s$ in the graph (including $s_0$, but excluding $s$); and
        \item $\ancestorsset_* \subseteq \ancestorsset$ is not empty and contains all the states of $\ancestorsset$ that have \textit{Kind} lower than $K(s)$.
    \end{itemize} 
	Considering the graph of a solution $\pi_*$ with $\cv(\pi_*) = \cv^*$.
\end{sublemma3}

\emph{Proof.} We use two nested induction to prove the statement above. 
The major (external) induction is decreasing on $K(s)$, with the base case when $K(s)$ is the maximum among the states in the graph of $\pi^*$. 
The minor (internal) induction is increasing on $d(s)$, being $d(s)$ the size of the longest directed simple $\pi_*$-trajectory in the graph of $\pi^*$ from $s$ to a state $s_D$, descendant of $s$ with $K(s_D) = K(s) - 1$, such that all intermediate states in the $\pi_*$-trajectory have \textit{Kind} equal to $K(s)$ (in other words, the longest $\pi_*$-trajectory from $s$ until reaching a state with decreased \textit{Kind}). Note that $g(s) + d(s) \leq \cv(\pi_*) = \cv^*$, by the formal definition of $\cv$s. We also note the above $n_D$ is an ancestral of $s$ contained in $\ancestorsset_*$, and that a state $s$ cannot have a successor state $s'$ with $K(s') < K(s) - 1$, by the formal definition of \textit{Kind}s.

\paragraph{Base Case.} We start analyzing when $K(s)$ is maximal. 

The \textit{base case} of the internal base case is when $d(s) = 1$. We prove this base case by contradiction, assuming that $\IDFSSearchRec(s, \ancestorsset, \ancestorsset_*, \pi)$ returns $\unsolved$ and does not decrease the $\newbound$ to a value not greater than $\cv^*$. Since $s$ is not in $(\ancestorsset \setminus \ancestorsset_*)$, the $\unsolved$ flag must have been returned in the last line of \IDFSSearchRec, meaning that it analyzed all actions applicable in $s$, and failed to find one that solves $s$, including the action $\pi_*(s)$. Let's see what happened when the for-loop analyzed the action $\pi_*(s)$.

We know that $\ancestorsset_* \neq \emptyset$, so the first if-continue statement will not be triggered. We also know $g(s) \leq \cv^* - d(s) = \cv^* - 1$, thus $g(s) + 1 \leq \cv^*$, meaning that the second if-continue statement will not be triggered as well, otherwise the $\newbound$ variable (which is never increased by \IDFSSearchRec) would be reduced to a value not greater than $\cv^*$, contradicting our initial hypothesis. Thus, we know that the repeat-loop was reached.

\ramon{Please, double check this part.}

Since the flag $\solved$ was not returned, we know that the recursive call on at least one successor state $s'$ of $s$ returned $\unsolved$. Since $d(s) = 1$, $K(s')$ cannot be equal to $K(s)$, otherwise $d(s) \geq d(s') + 1 \geq 1 + 1$ (contradicting $d(s) = 1$). Then, we know that $K(s') = K(s) - 1$, and thus $s'$ is covered by $\ancestorsset_*$, therefore the recursive call would immediately return $\solved$, what is a contradiction, concluding our proof by contradiction.~$\hfill\circ$

Now, we analyze the \textit{induction step} of the internal base case, when $d(s) > 1$. We prove this induction step by contradiction, and, base on the same arguments we used for the base case, we find that the repeat-loop was reached for the action $\pi_*(s)$, as well that the recursive call on at least one successor state $s'$ of $s$ returned $\unsolved$.

We know that $K(s') = K(s)$, otherwise $s'$ would be in $\ancestorsset_*$, and the recursive call would immediately return $\solved$, what would be a contradiction. Then, we can apply the minor inductive hypothesis in $s'$, proving that $\IDFSSearchRec(s', \ancestorswiths, \ancestorsset_*' \supseteq \ancestorsset_*, \pi' \supseteq \pi)$ either returns $\solved$ or decreases the $\newbound$ to a value not greater than $\cv^*$. The first option is false because it would cause a direct contradiction. The second one is false as well because the $\newbound$ variable has its value never increased by \IDFSSearchRec, and our initial hypothesis was that $\IDFSSearchRec(s, \ancestorsset, \ancestorsset_*, \pi)$ does not decrease the $\newbound$ to a value not greater than $\cv^*$. This concludes our proof by contradiction.~$\hfill\circ$

$\hfill\square$

\paragraph{Induction Step.} 
For the induction step, we assume that $K(s)$ is not maximal, thus we have to consider that some successor states $s'$ of $s$ may have $K(s') > K(s)$, what was't possible before.

The \textit{base case} of the internal induction step is when $d(s) = 1$. We prove this base case by contradiction, and by the same arguments again we find that the repeat-loop was reached for the action $\pi_*(s)$, as well that the recursive call on at least one successor state $s'$ of $s$ returned $\unsolved$.

If $K(s') = K(s) - 1$, the proof is the same as for the base case of the internal base case, so we disregard that case. $K(s')$ again cannot be equal to $K(s)$ (otherwise contradicting $d(s) = 1$). So $K(s')$ must be greater than $K(s)$.

We know that $s$ has at least one successor $s''$ that has $K(s'') \leq K(s)$, otherwise, there would be no trail $t$ with $K(t) = K(s)$ including $s$. And by the arguments of the previous paragraph, we know that $s''$ has $K(s'') = K(s) - 1$, and, by using the same proof as for the base of the base case, we also know that the recursive call on $s''$ returns the $\solved$ flag. Thus, we know that at some point in the repeat-loop, the recursive call on $s'$ had $\ancestorsset_*' = \ancestorswiths$. Now, if we apply the major inductive hypothesis, we know that $\IDFSSearchRec(s', \ancestorswiths, \ancestorsset_*' = \ancestorswiths, \pi' \supseteq \pi)$ either returns $\solved$ or decreases the $\newbound$ to a value not greater than $\cv^*$. The first option is false because it would cause a direct contradiction. The second as well, using the same argument as for the induction step of the base case. Thus we conclude our proof by contradiction.~$\hfill\circ$

Now, we analyze the \textit{induction step} of the internal induction step, that is when $d(s) > 1$.  We will also follow with a proof by contradiction, and by the same arguments again we find that the repeat-loop was reached for the action $\pi_*(s)$, as well that the recursive call on at least one successor state $s'$ of $s$ returned $\unsolved$.

There are three cases for $K(s')$: $K(s') = K(s) - 1$,  $K(s') = K(s)$, or  $K(s') > K(s)$. For the first case, we can apply the argument used in the base case of the internal base case to get a contradiction. For the second case, we can apply the argument used in the induction case of the internal base case to get a contradiction. For the third case, we can apply the argument used in the base case of the internal induction case to get a contradiction. Thus, by exhaustion, we proved a contradiction for the induction case of the induction case as well, concluding the proof of this Lemma.~$\hfill\circ$

$\hfill\square$

$\hfill\blacksquare$

\newpage

%------------------------------------------------------------------------
\subsection*{Conclusion}

Finally, with the Claims~1 and~2, and Lemmas~\ref{lem:increasing_bound},~\ref{lem:no_false_positives} and~\ref{lem:no_false_negatives} properly in place and proved, we formally prove that our \IDFSSearch algorithm is sound and complete, as follows.

\begin{theorem}
The algorithm \IDFSSearch is sound and complete.
\end{theorem}
\emph{Proof.} Claims~1 and~2 combined assert that, if Lemmas~\ref{lem:increasing_bound},~\ref{lem:no_false_positives} and~\ref{lem:no_false_negatives} are true, then the \IDFS algorithm (Algorithm~\ref{alg:IDFS}) is \textbf{sound} and \textbf{complete}.~$\hfill\blacksquare$
